# Supplementary material for: Longitudinal Deep Kernel Gaussian Process Regression
Source: arXiv:2005.11770 source file (2020-12-07)
Supplement: Supplementary file 1 [file appendix.tex]

\section*{A. Derivations for L-DKGPR}
\label{app:derivations}
\para{Model Inference.}
We start with the ELBO:
\begin{linenomath}
\begin{equation}
\label{appeq:elbo}
    \mathcal{L}\triangleq \mathbb{E}_{q(\tf,\tu|X,Z)}[\log p(\by|\tf)]-\text{KL}[q(\tu|X,Z)||p(\tu|Z)]
\end{equation}
\end{linenomath}

where $q(\tf,\tu|X,Z)=p(\tf|\tu,X,Z) q(\tu|X,Z)$. Following the DTC assumption \cite{liu2020gaussian}, we substitute $p(\tf|\tu,X,Z)$ with its deterministic form $\tf=A\tu$ with $A=K_{XZ}K_{ZZ}^{-1}$. Together with the reparameterization $q(\tu|X,Z)=\bmu_q+L_q \bep$ with $\bep{\sim}\mathcal{N}(\bm{0},I)$, we can rewrite the first term of \eqref{appeq:elbo} as:
\begin{linenomath}
\begin{align}
\label{appeq:variational_posterior}
    \nonumber
    & \mathbb{E}_{q(\tf,\tu|X,Z)}[\log p(\by|\tf)] \\ \nonumber
    = & -N\log \sigma - \frac{1}{2\sigma^2}\mathbb{E}_{\bep}[\Norm{\by - A(\bmu_q + L_q\bep))}^2_2] \\
    =& -N \log \sigma - \frac{1}{2\sigma^2}\left(\Norm{\by}_2^2-2\by^\top A\bmu_{q} + \Norm{A\bmu_{q}}_2^2 + \Norm{A L_q \bm{1}}_2^2\right)
\end{align}
\end{linenomath}

Since the second term in \eqref{appeq:elbo} is the KL divergence between two multivariate Gaussian distributions, the analytical form can be obtained directly as
\begin{linenomath}
\begin{align}
\label{appeq:kl} \nonumber
    2\text{KL}(q(\tu|X,Z)& ||p(\tu|Z)) = \log \frac{\norm{K_{ZZ}}}{\norm{L_q}^2} \\
    & - M + \text{tr}(K_{ZZ}^{-1} L_q L_q^\top) + \bm{\mu}_q^\top K_{ZZ}^{-1} \bm{\mu}_q
\end{align}
\end{linenomath}

Combining \eqref{appeq:variational_posterior} and \eqref{appeq:kl}, we therefore obtain:
\begin{linenomath}
\begin{align}
\label{appeq:elbo_ana}
\nonumber
    \mathcal{L} = &\underbrace{-N\log\sigma - \frac{1}{2\sigma^{2}} \left(\Norm{\by}_2^2-2\by^\top A\bmu_{q} + \Norm{A\bmu_{q}}_2^2 + \Norm{A L_q \bm{1}}_2^2\right)}_{\mathbb{E}_{q(\tf,\tu|X,Z)}[\log p(\by|\tf)]} \\ 
    & -\underbrace{\frac{1}{2}\left[\log \frac{\norm{K_{ZZ}}}{\norm{L_q}^2}
    - M + \text{tr}(K_{ZZ}^{-1}L_q L_q^\top) + \bm{\mu}_q^\top K_{ZZ}^{-1} \bm{\mu}_q\right]}_{\text{KL}[q(\tu|X,Z)||p(\tu|Z)]}
\end{align}
\end{linenomath}
where $\bm{1}$ is a column vector of ones. We can then compute the partial derivatives of $\mathcal{L}$ w.r.t. the parameters of the proposal posterior $q(\tu|X,Z)$ (\ie $\{\bmu_q, L_q\}$) and derive its optimal form, such that:
\begin{linenomath}
\begin{align}
    & \frac{\partial \mathcal{L}}{\partial \bmu_q}=\frac{1}{\sigma^2}(-A^\top \by + A^\top A \bmu_q) + K_{ZZ}^{-1}\bmu_q = 0 \\
    & \frac{\partial \mathcal{L}}{\partial L_q} = \frac{1}{\sigma^2}A^\top A L_q \bm{1}\bm{1}^\top + (L_q^{-\top} + K_{ZZ}^{-1}L_q) = 0
\end{align}
Solving the above equations gives:
\begin{align}
    & \bmu_q = \sigma^{-2}K_{ZZ}BK_{XZ}^\top \by \label{appeq:muq}\\
    & L_q(\tI + \bm{1}\bm{1}^\top) = K_{ZZ}BK_{ZZ} \label{appeq:lq}
\end{align}
\end{linenomath}
with $B=(K_{ZZ} + \sigma^{-2}K_{XZ}^\top K_{XZ})^{-1}$. To solve the triangular matrix $L_q$ from \eqref{appeq:lq}, we first compute the Cholesky decomposition of $\tI+\bm{1}\bm{1}^\top = CC^\top$ and $K_{ZZ}BK_{ZZ} = UU^T$. We then simplify both side of \eqref{appeq:lq} to $L_qC = U$. $L_q$ can then be solved by exploiting the triangular structure on both side with
\begin{linenomath}
\begin{align}
\label{appeq:lq_solve}
    L_{i,i-k}= \frac{U_{i,i-k}-\sum_{j=0}^{k-1}L_{i,i-j}C_{i-j,i-k}}{C_{i-k,i-k}}, && k=0,1,\cdots,i-1
\end{align}
\end{linenomath}
where $L_{i,j}$ is a short notation for $[L_q]_{i,j}$. 

\para{Prediction.}
A common approximation assumption associated with the inducing points idea is that the signals between training data and test data are conditionally independent given $\tu$ \cite{quinonero2005unifying}. This is particularly useful during the test phase. Given the covariate matrix $\Xstar$ for the test data, the prediction distribution is given by:
\begin{linenomath}
\begin{align}
\label{appeq:predictive_londkgp}
    p(\tf_*|\Xstar,X,y,Z) &= \int p(\tf_*,\tf,\tu|\Xstar,X,y,Z) d\tf d\tu \nonumber\\
    &= \int p(\tf_*|\tu,X_*,Z) p(\tf,\tu|X,y,Z) d\tf d\tu \nonumber\\
    &\simeq \mathbb{E}_{q(\tu|X,Z)}[p(\tf_*|\tu,X_*,Z)] \nonumber \\ \nonumber
    &= \mathcal{N}(K_{\Xstar Z}[K_{ZZ}+\sigma^2 \tI]^{-1}\bm{\mu}_q,\\
    &K_{\Xstar \Xstar} - K_{\Xstar Z}[K_{ZZ}+\sigma^2 \tI]^{-1}K_{\Xstar Z}^\top)
\end{align}
\end{linenomath}
We can then make prediction using the mode and evaluate the prediction uncertainty with the covariance matrix from \eqref{appeq:predictive_londkgp}.

\section*{B. Implementation Details and Parameter Setup}
\label{app:implementation_details}
We implement L-DKGPR using PyTorch \cite{NEURIPS2019_9015}. We formulate $e_\gamma$ using a deep neural network (DNN) consisting of multiple fully connected layers. Specifically, the structure of $e_\gamma$ is \texttt{$P$-$H$-CELU-D(0.2)-$H$-CELU-D(0.2)-$D_v$}, where $H$ is the size of hidden units, \texttt{CELU} stands for Continuously Differentiable Exponential Linear Units \cite{barron2017continuously} and \texttt{D(0.2)} represents a dropout layer with 20\% dropout rate. We set $H=16$ for simulated data and $H=32$ for real-life data. The latent dimension $D_v$ is fixed at $10$ for all experiments. Although we only use a simple fully connected structure throughout the experiment, the implementation is flexible enough to allow more advanced DNN structure such as CNN and RNN. The embedding function $g_\phi$ is a $I$-by-$D_i$ parameter matrix. We set $D_i=D_v$. Though the full lower triangular matrix $L_q$ can be computed using \eqref{appeq:lq_solve}, we find that approximating $L_q$ by using only its main diagonal components provides similar accuracy, but have substantially less computation and numerically stable. Therefore, in our implementation, $\tilde{L_q}=\text{diag}(U/C)$. We update $\Theta=\{\sigma^2, Z,\alpha^{(v)},\alpha^{(i)}, \gamma, \phi\}$ using Adam optimizer. The learning rate for $\Theta-\{\phi\}$ is fixed at $0.001$. To facilitate more effective learning on cluster correlation, we assign larger learning rate on $\{\phi\}$, which is fixed at $0.01$. The training and testing batch sizes are set to $1024$. The maximum training epoch of L-DKGPR is set to 300 for all data sets. We use early stopping if the R$^2$ evaluated on validation set decrease in two consecutive epochs. The number of Inducing points is fixed at $10$ for all data sets. We initialize $\{\sigma^2,\alpha^{(v)},\alpha^{(i)}\}=1$, $Z{\sim}U[0,1)^{M\times (D_v+D_i)}$. $\gamma,\phi$ are initialized with the default initialization mechanism in PyTorch. To avoid numerical issue during Cholesky decomposition, we add a small factor $\Delta=\text{diag}(\bm{0.001})$ to the main diagonal of the correlation matrix.

As for the implementation of our baseline methods, we use the implementations of GLMM, GEE and LGPR available in the \texttt{lmer4}, \texttt{PGEE} and \texttt{lgpr} packages, respectively from CRAN.\footnote{\url{https://cran.r-project.org/}}. We use the LMLFM implementation  from \url{https://github.com/junjieliang672/LMLFM}. Implementation of ODVGP and KISSGP can be found through Gpytorch \cite{gardner2018gpytorch}. For GLMM, we keep most hyper-parameters to their default values but increase the maximum iteration to 200. In GEE, we use an first-order auto-regressive correlation structure. The maximum iteration is fixed at 200. For LGPR, results are averaged over 5 independent simulated chains. For each chain, we use 2000 iterations. The number of burn-in samples is fixed at 200. Performance of ODVGP seems to be sensitive to the the initialization of the inducing points. We find that using the cluster centers learned by a KMeans algorithm generally produce more stable results. Throughout all experiments, the number of inducing points for both mean and variance are fixed at 100. We use the same deep encoder as used in L-DKGPR for KISSGP. The number of inducing points for KISSGP is fixed at 32. Maximum iteration for both ODVGP and KISSGP is fixed at 200.

All experiments are conducted on a desktop machine with Intel Core i7-7700K CPU, 32GB RAM and RTX 2070 super graphics card. Codes are available through \url{https://anonymous.4open.science/r/cce1f2c6-29ff-4941-993d-d597a71ecc8c/}.

\section*{C. Experimental Data Setup}
\label{app:setup}
\para{Generating Simulated Data.}
We construct simulated longitudinal data sets that exhibit  \ie longitudinal correlation (LC) and multilevel correlation (MC) as follows: The outcome is generated using $\by=f(X)+\bm{\epsilon}$ where $f(X)$ is a non-linear transformation based on the observed covariate matrix $X$ and the residual $\bm{\epsilon}{\sim}N(\bm{0},\Sigma)$. To simulate longitudinal correlation, we simply set $\Sigma$ to a block diagonal matrix. For each individual, we use a  first-order auto-regressive correlation structure ($\text{AR}(1)$) with decaying factor fixed at $0.9$. To simulate a data set that exhibits multilevel correlation, we first split the individuals into $C$ clusters. We then define the cluster correlation matrix by setting the correlation associated to data points in the same cluster to $1$. Finally, we compute the multilevel correlation by summing up the longitudinal correlation and cluster correlation. Following  \cite{cheng2019additive,timonen2019interpretable}, we simulate $40$ individuals, $20$ observations, and $30$ covariates for each individual. To simulate correlation among the covariates, we first generate $10$ base features independently from $[0,1)$ uniform distribution, then the covariate matrix $X$ is computed using an encoder network with architecture $10-100-Tanh-Dropout(0.7)-BatchNorm-30-Tanh$. It therefore results in 30 covariates that are conditionally independent given encoder network and base features. We hold out both the base features and the encoder network to all comparing methods, thus leading to a covaraite matrix with non-linear correlation that is unknown to all methods. To generate $\by$, we use another nonlinear transformation $f(X)$, which is defined by a network with structure $30-100-Tanh-1$. In our experiment, We vary the number of clusters $C$ from $[2,5]$.

\para{Pre-processing on SWAN data.}
Since CESD score is not contained from the original SWAN data, we manually compute the score based on its definition \cite{radloff1977ces}. To form the outcome label, we define an adjusted CESD score by $y=CESD-15$, thus $y\geq 0$ indicates depression. We center $\by$ with $\by=\by-\text{mean}(\by)$. After computing the label, we exclude all columns that are directly associated to computing the CESD score. We convert the categorical features using one-hot encoding and perform standard scaling on the continuous features. 

\para{Pre-processing on GSS data.}
Since the original data set contains repeated columns for the same survey question, we keep only one column for each survey question. We re-format all the answer codes associated to `unknown' and `missing' to `unknown'. The outcome label is derived from the field `General Happiness', we code the value `pretty happen' and `very happy' to $1$ and the others to $-1$. As the other covaraites, We convert the categorical features using one-hot encoding and perform standard scaling on the continuous features. 

\para{Pre-processing on TADPOLE data.}
There are three data sets in the original files. We first combine the three data sets and remove the repeated data points. Then, we convert the categorical features using one-hot encoding and perform standard scaling on the continuous features. The outcome label is defined by the value of `ADAS13'. Similarly, we center the label with $\by=\by-\text{mean}(\by)$.

\section*{D. Additional Experiment Results}
\label{app:additional_exp}
\subsection{Run time Comparison}
\label{app:runtime}
The CPU run times and failure to complete execution on the real-world data sets are reported in \ref{apptab:real_life}. We see that LGPR, GLMM and GEE are exceptionally sensitive to the number of variables. Indeed, their computational complexity increases proportional to $P^3$ where $P$ is the number of variables. In contrast, L-DKGPR, LMLFM and state-of-the-art GP baselines  (KISSGP and ODVGP) scale gracefully with increasing number of data points and covariates.

\begin{table*}[tb]
\small
\caption{Runtime (in second) comparison on real-world data sets. We use `N/A' to denote execution error.}
\begin{center}
\begin{tabular}{cccc|ccccccc}
\toprule
Data sets & $N$ & $I$ & $P$ & L-DKGPR & KISSGP & ODVGP & LGPR           & LMLFM        & GLMM         & GEE  \\
\midrule
TADPOLE                    & 595   & 50                   & 24    & 0.03 & 0.34 & 0.03  & 6.39 & 0.01  & 0.01 & 0.13\\
SWAN                       & 550    & 50                   & 137                      & 0.03 & 0.29 &  0.04 & 26.1 & 0.02  & 0.06 & 0.59      \\
GSS                        & 1,500  & 50                   & 1,553   & 0.12 & 0.09 & 0.11 & N/A  & 0.30  & N/A     & 30.1 \\ \hline

TADPOLE                    & 8,771  & 1,681                & 24          & 1.48 & 0.36 &   1.32  & N/A     & 0.25  & 0.03 & 4.66\\
SWAN                       & 28,405 & 3,300                & 137               & 4.48  & 1.21 &  2.81 & N/A  & 1.74  & N/A  & N/A    \\
GSS                        & 59,599 & 4,510                & 1,553               & 5.31 & 2.01 & 4.65 & N/A  & 24.35 & N/A  & N/A  \\
\bottomrule
\end{tabular}
\end{center}
\label{apptab:real_life}
\end{table*}

\subsection{Correction Structure in Simulated Data.}
\label{app:rq3}
\begin{figure*}[t!]
\centering 
\includegraphics[width=.9\linewidth]{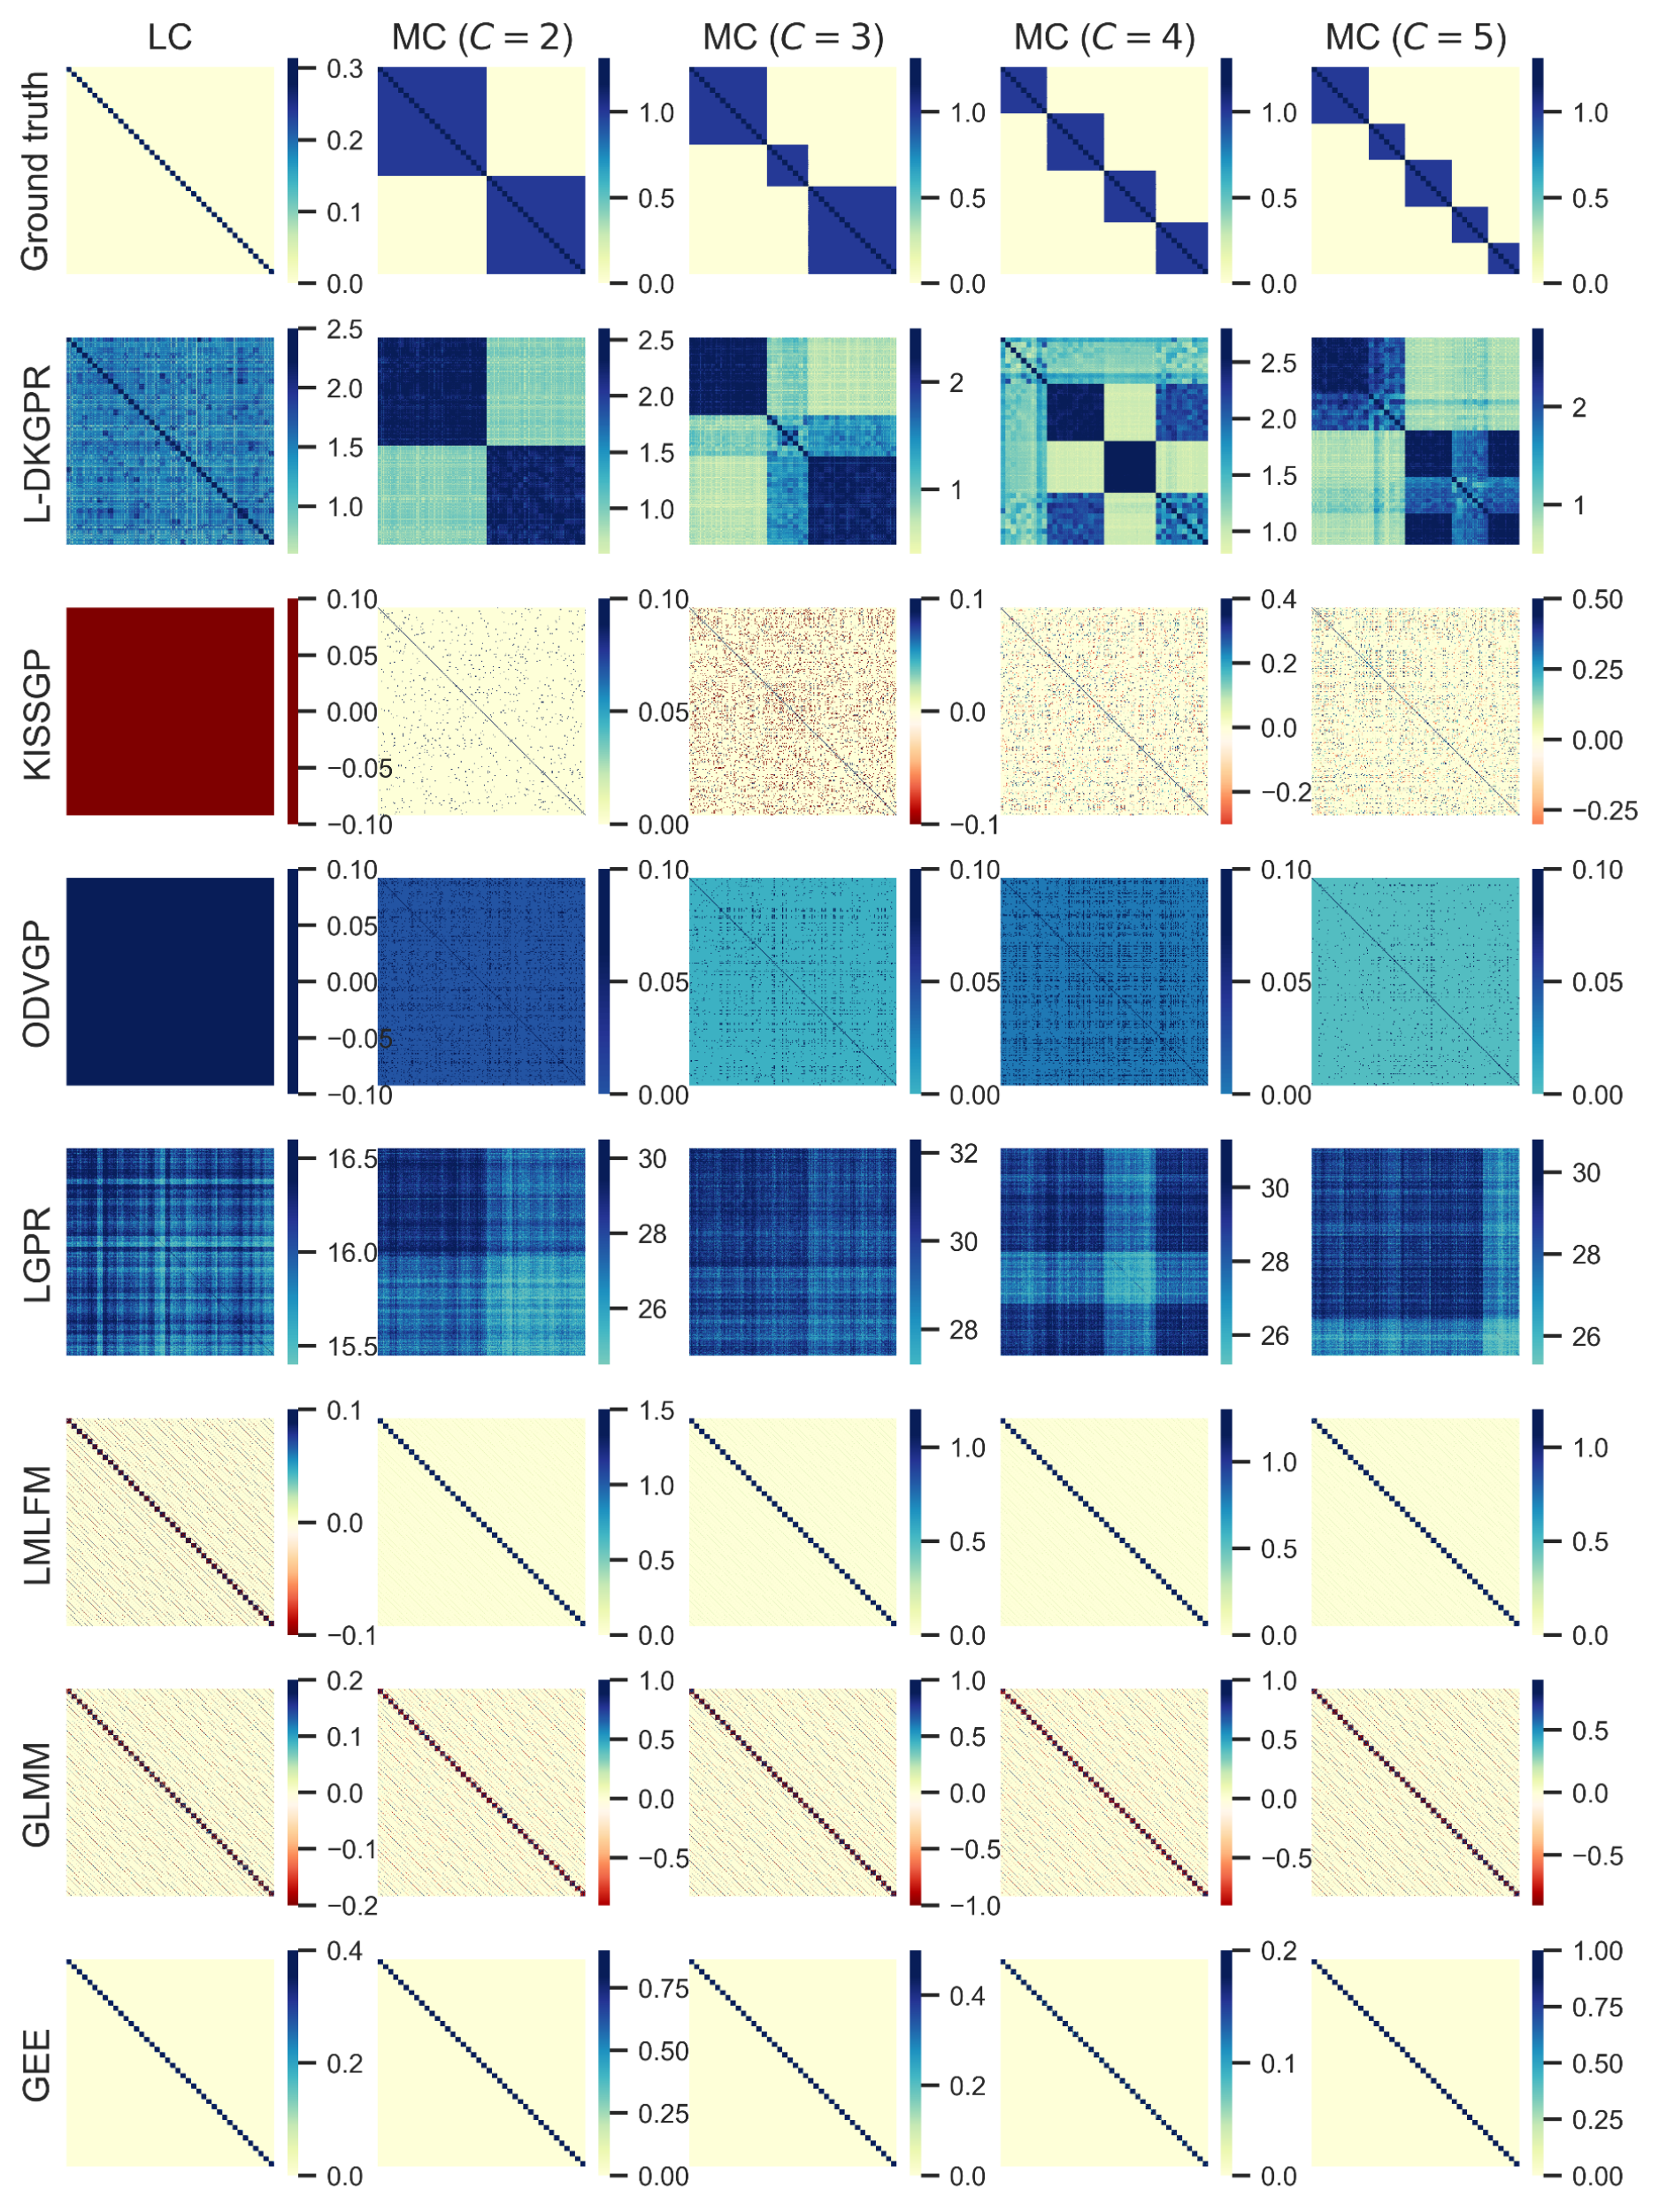}
\caption{Outcome correlation estimated by all methods on simulated data.}
\label{appfig:corr_compare}
\end{figure*}

The outcome correlations estimated by all methods on the simulated data are shown in Figure~\ref{appfig:corr_compare}. 
It is easy to see that KISSGP and ODVGP are incapable of recovering any correlation structure from the data. LGPR seems to be slightly better than KISSGP and ODVGP when MC is presented. However, we see that only one known cluster is correctly recovered when $C>2$. The correlation estimation results also justify the inferior regression performance in terms of $\text{R}^2$ as they fail to learn the correlation structure.
Moreover, we see that LMLFM, GLMM and GEE are only capable of recovering LC, but not MC. This fact is quite reasonable since by design LMLFM is only able to handle a special case of MC where cluster correlation exists for individuals observe at the same time. Both GLMM and GEE rely on a correct input of correlation structure which is assumed a priori unknown. We note that L-GKDPR is able to recover most of the correlation structure present in the data. We further note that L-DKGPR, despite being the best performer among the methods compared in this study, it tends to underestimate the number of clusters because  the full data correlation is approximated by a low-rank matrix (see Eq.~\eqref{appeq:predictive_londkgp}) resulting in information loss.

\subsection{Case Study: Correction Structure in SWAN Data.}
\label{app:rq3_case_study}
\begin{figure*}[t]
\centering 
\subfigure[Cluster Correlation]{
\includegraphics[width=.42\linewidth]{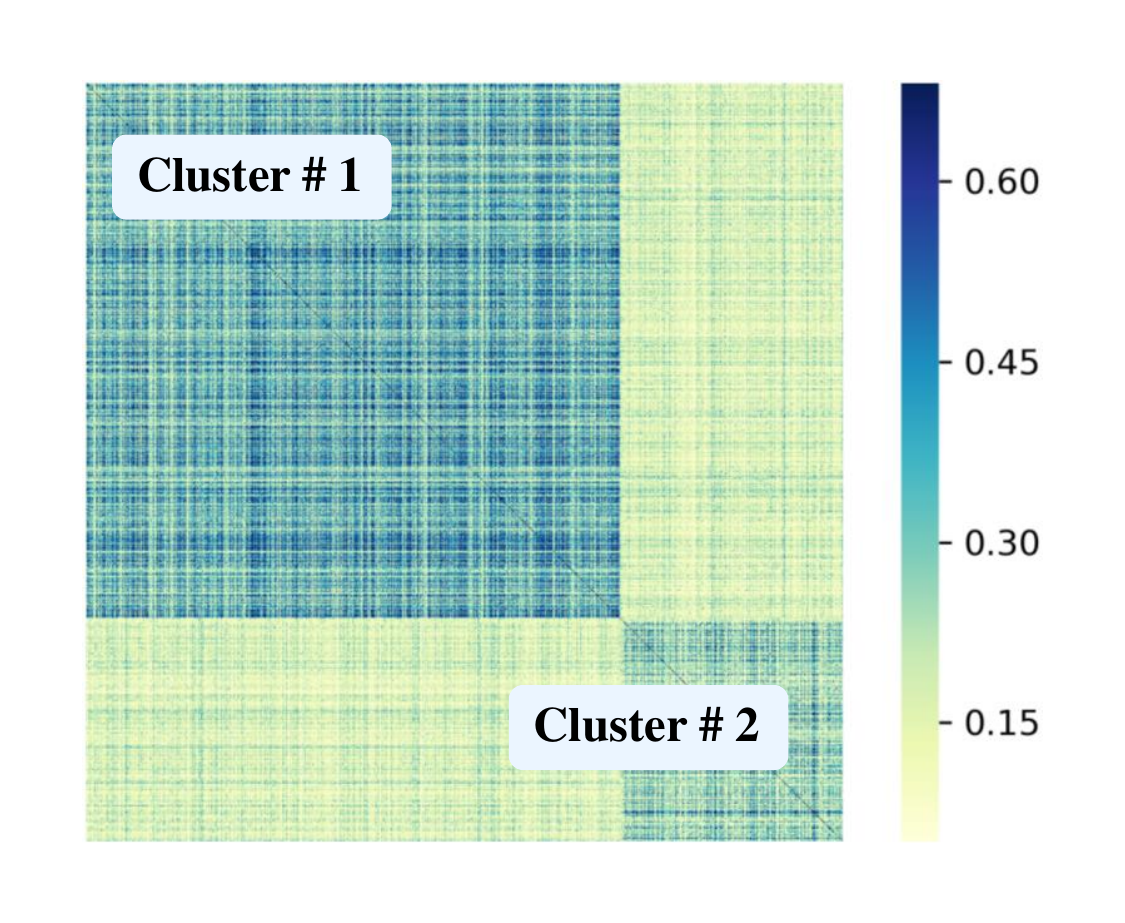}
\label{appfig:swan_cluster_corr} 
}
\subfigure[Score Density]{
\includegraphics[width=.42\linewidth]{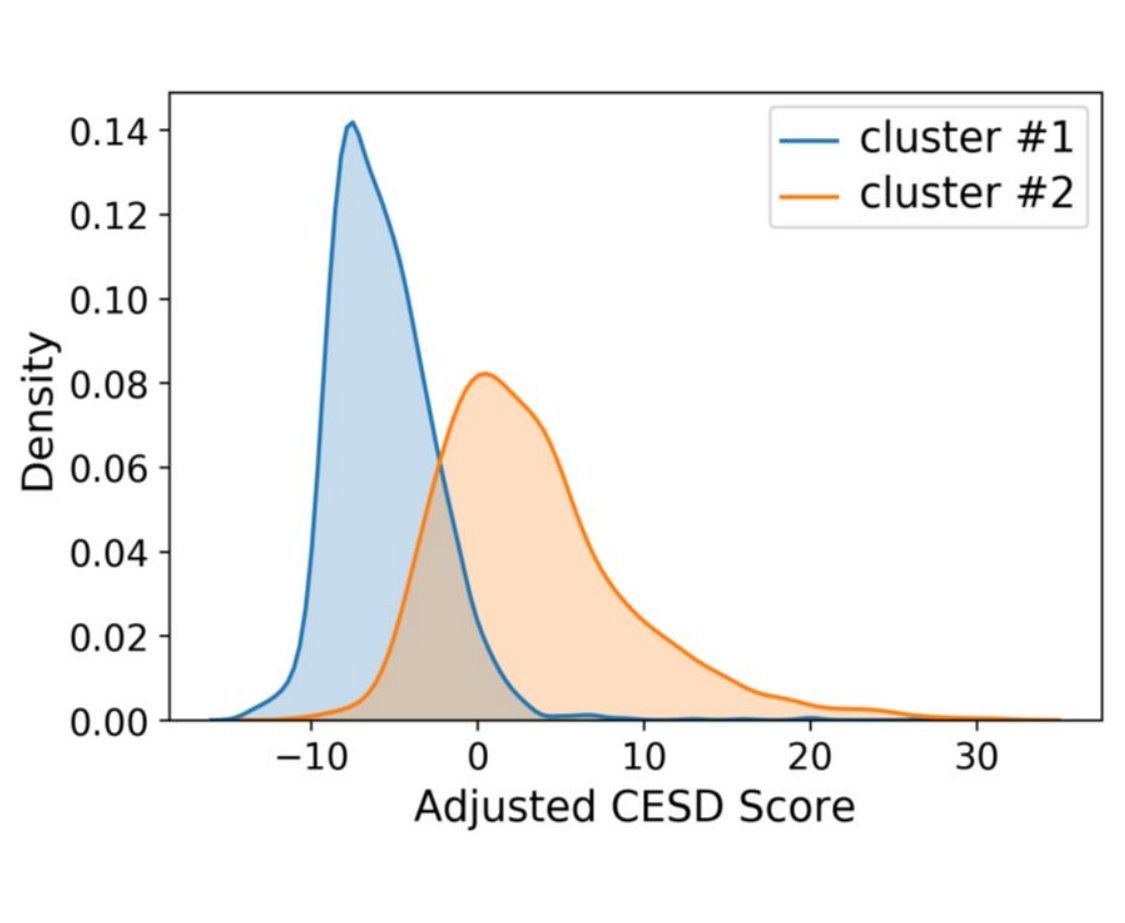}
\label{appfig:swan_cluster_density}
}
\caption{Cluster correlation analysis on SWAN Data. 
% (a) We find that individuals can be roughly split into two clusters; (b) Adjusted CESD score density for the two clusters.
}
\label{appfig:swan_cluster}
\end{figure*}

\begin{figure*}[t!]
\centering 
\subfigure[Individual \#1]{
\includegraphics[width=.45\linewidth]{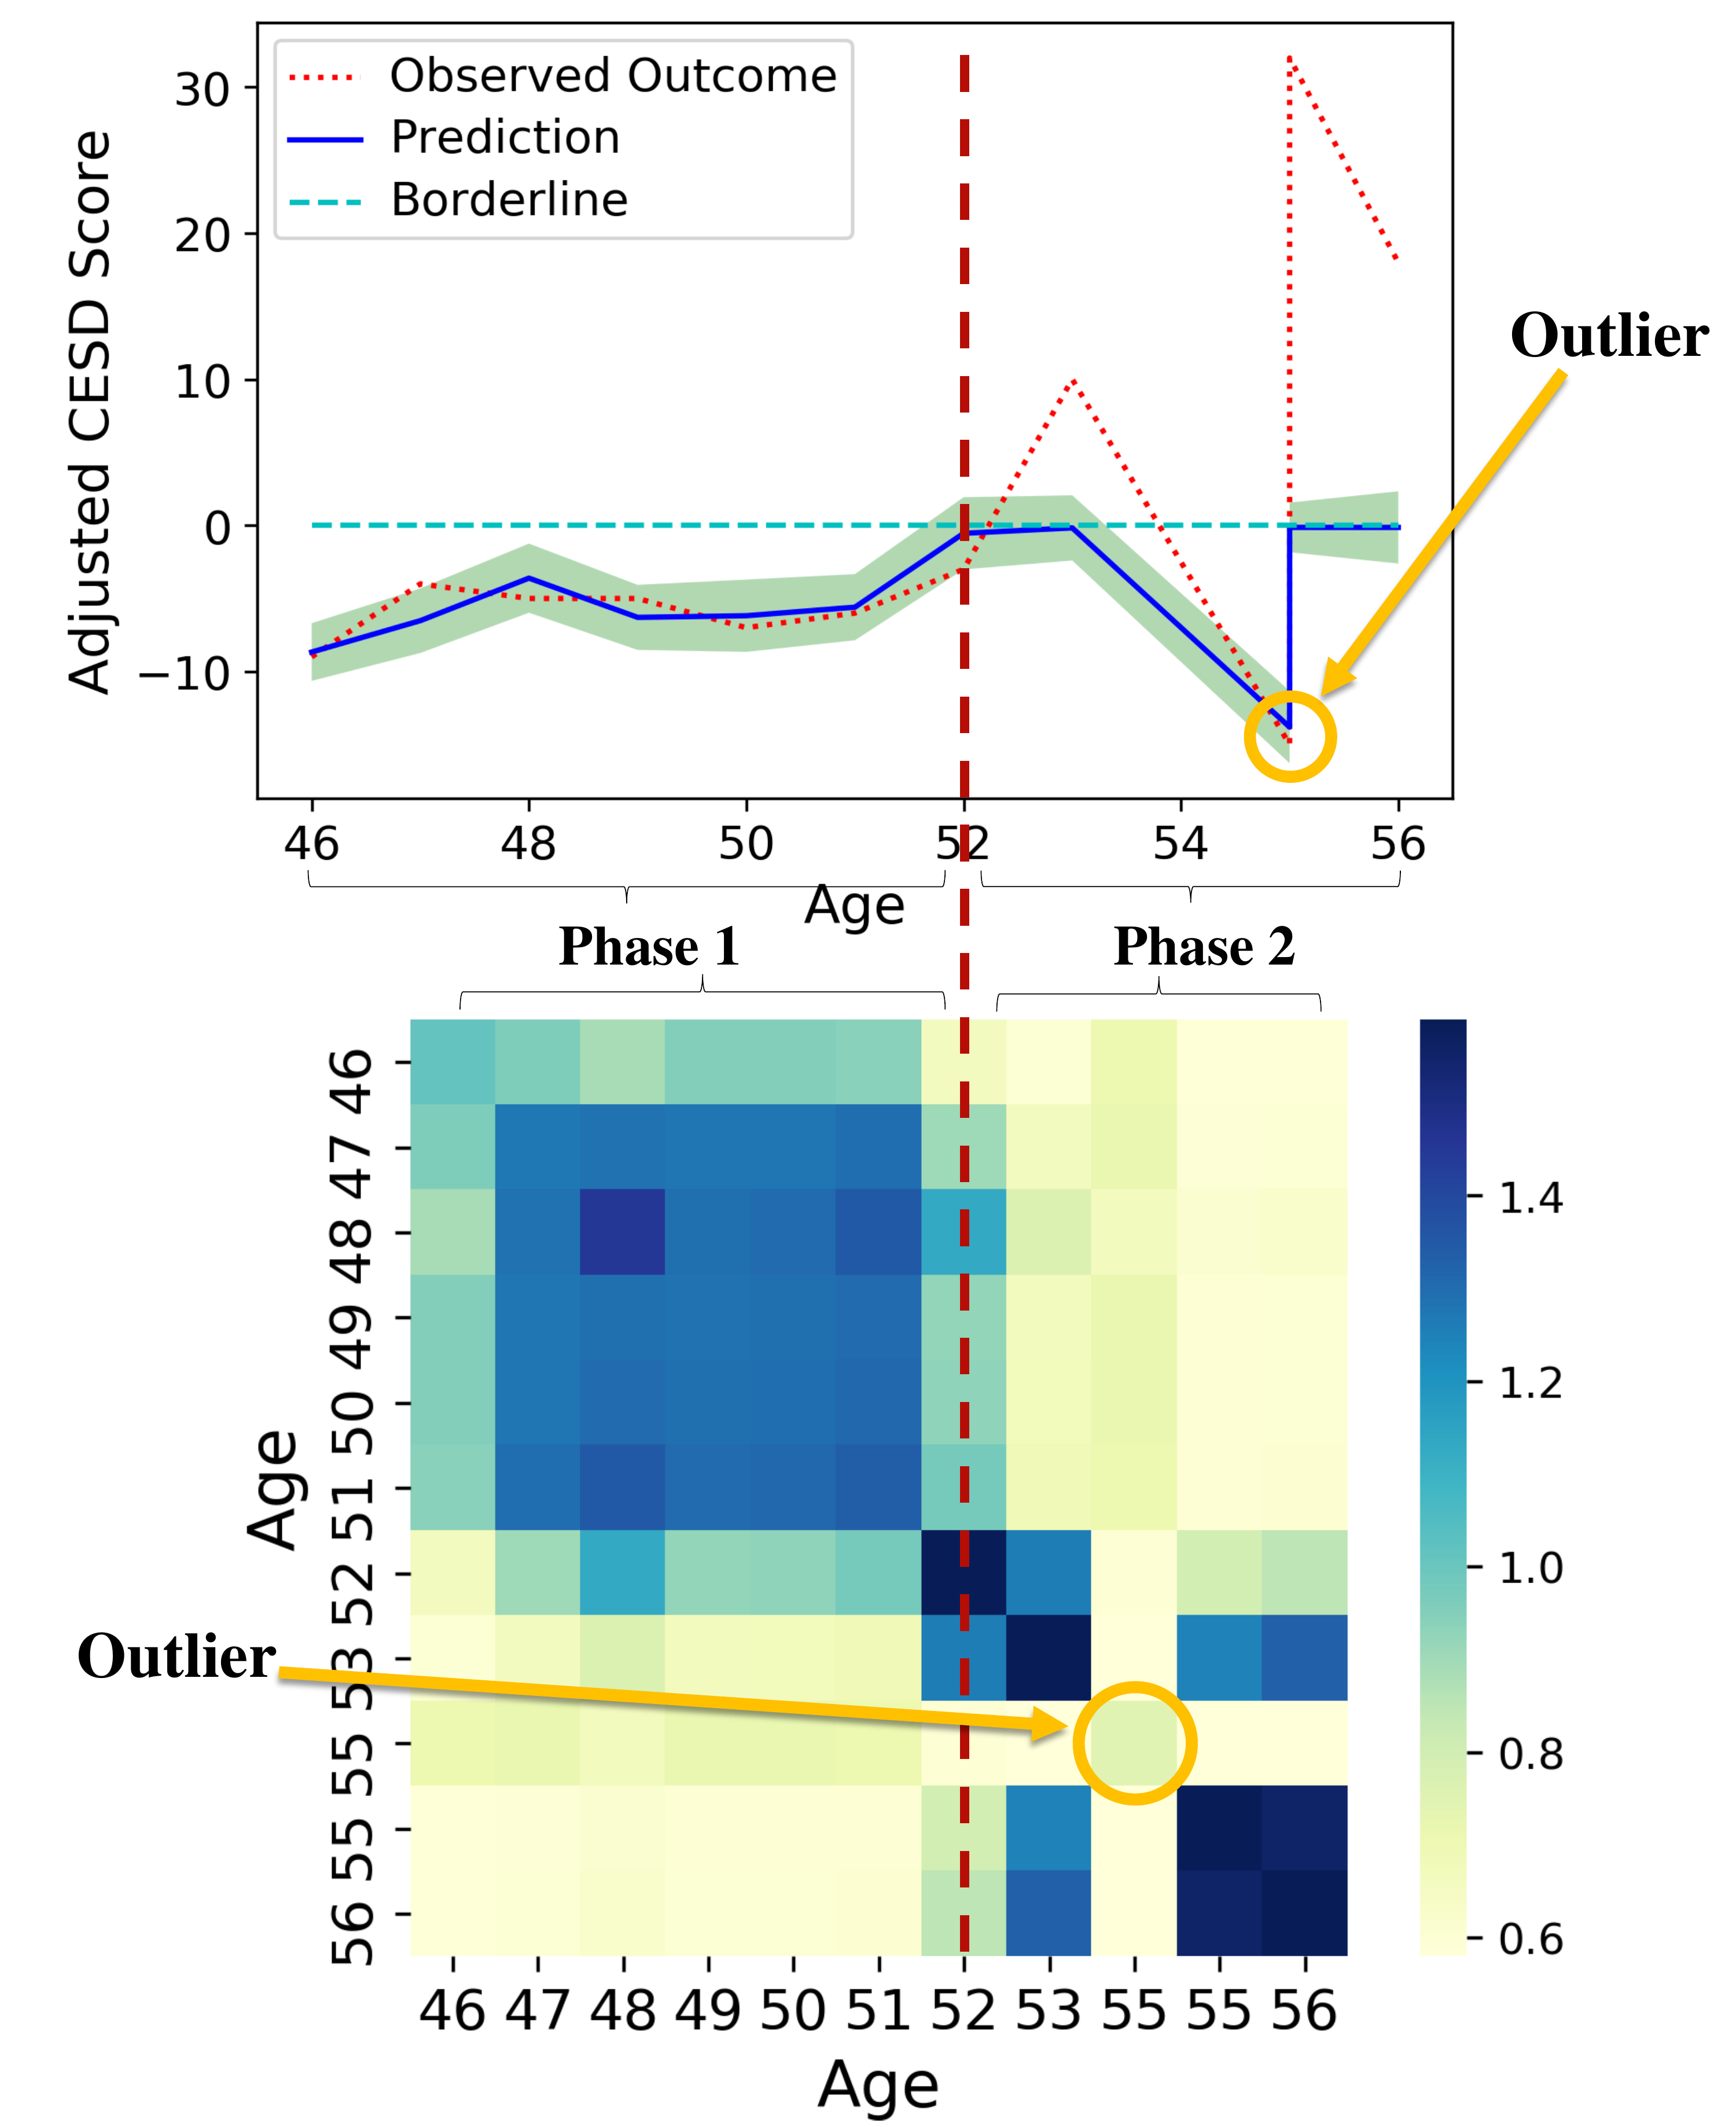}
\label{appfig:individual1} 
}
\subfigure[Individual \#2]{
\includegraphics[width=.45\linewidth]{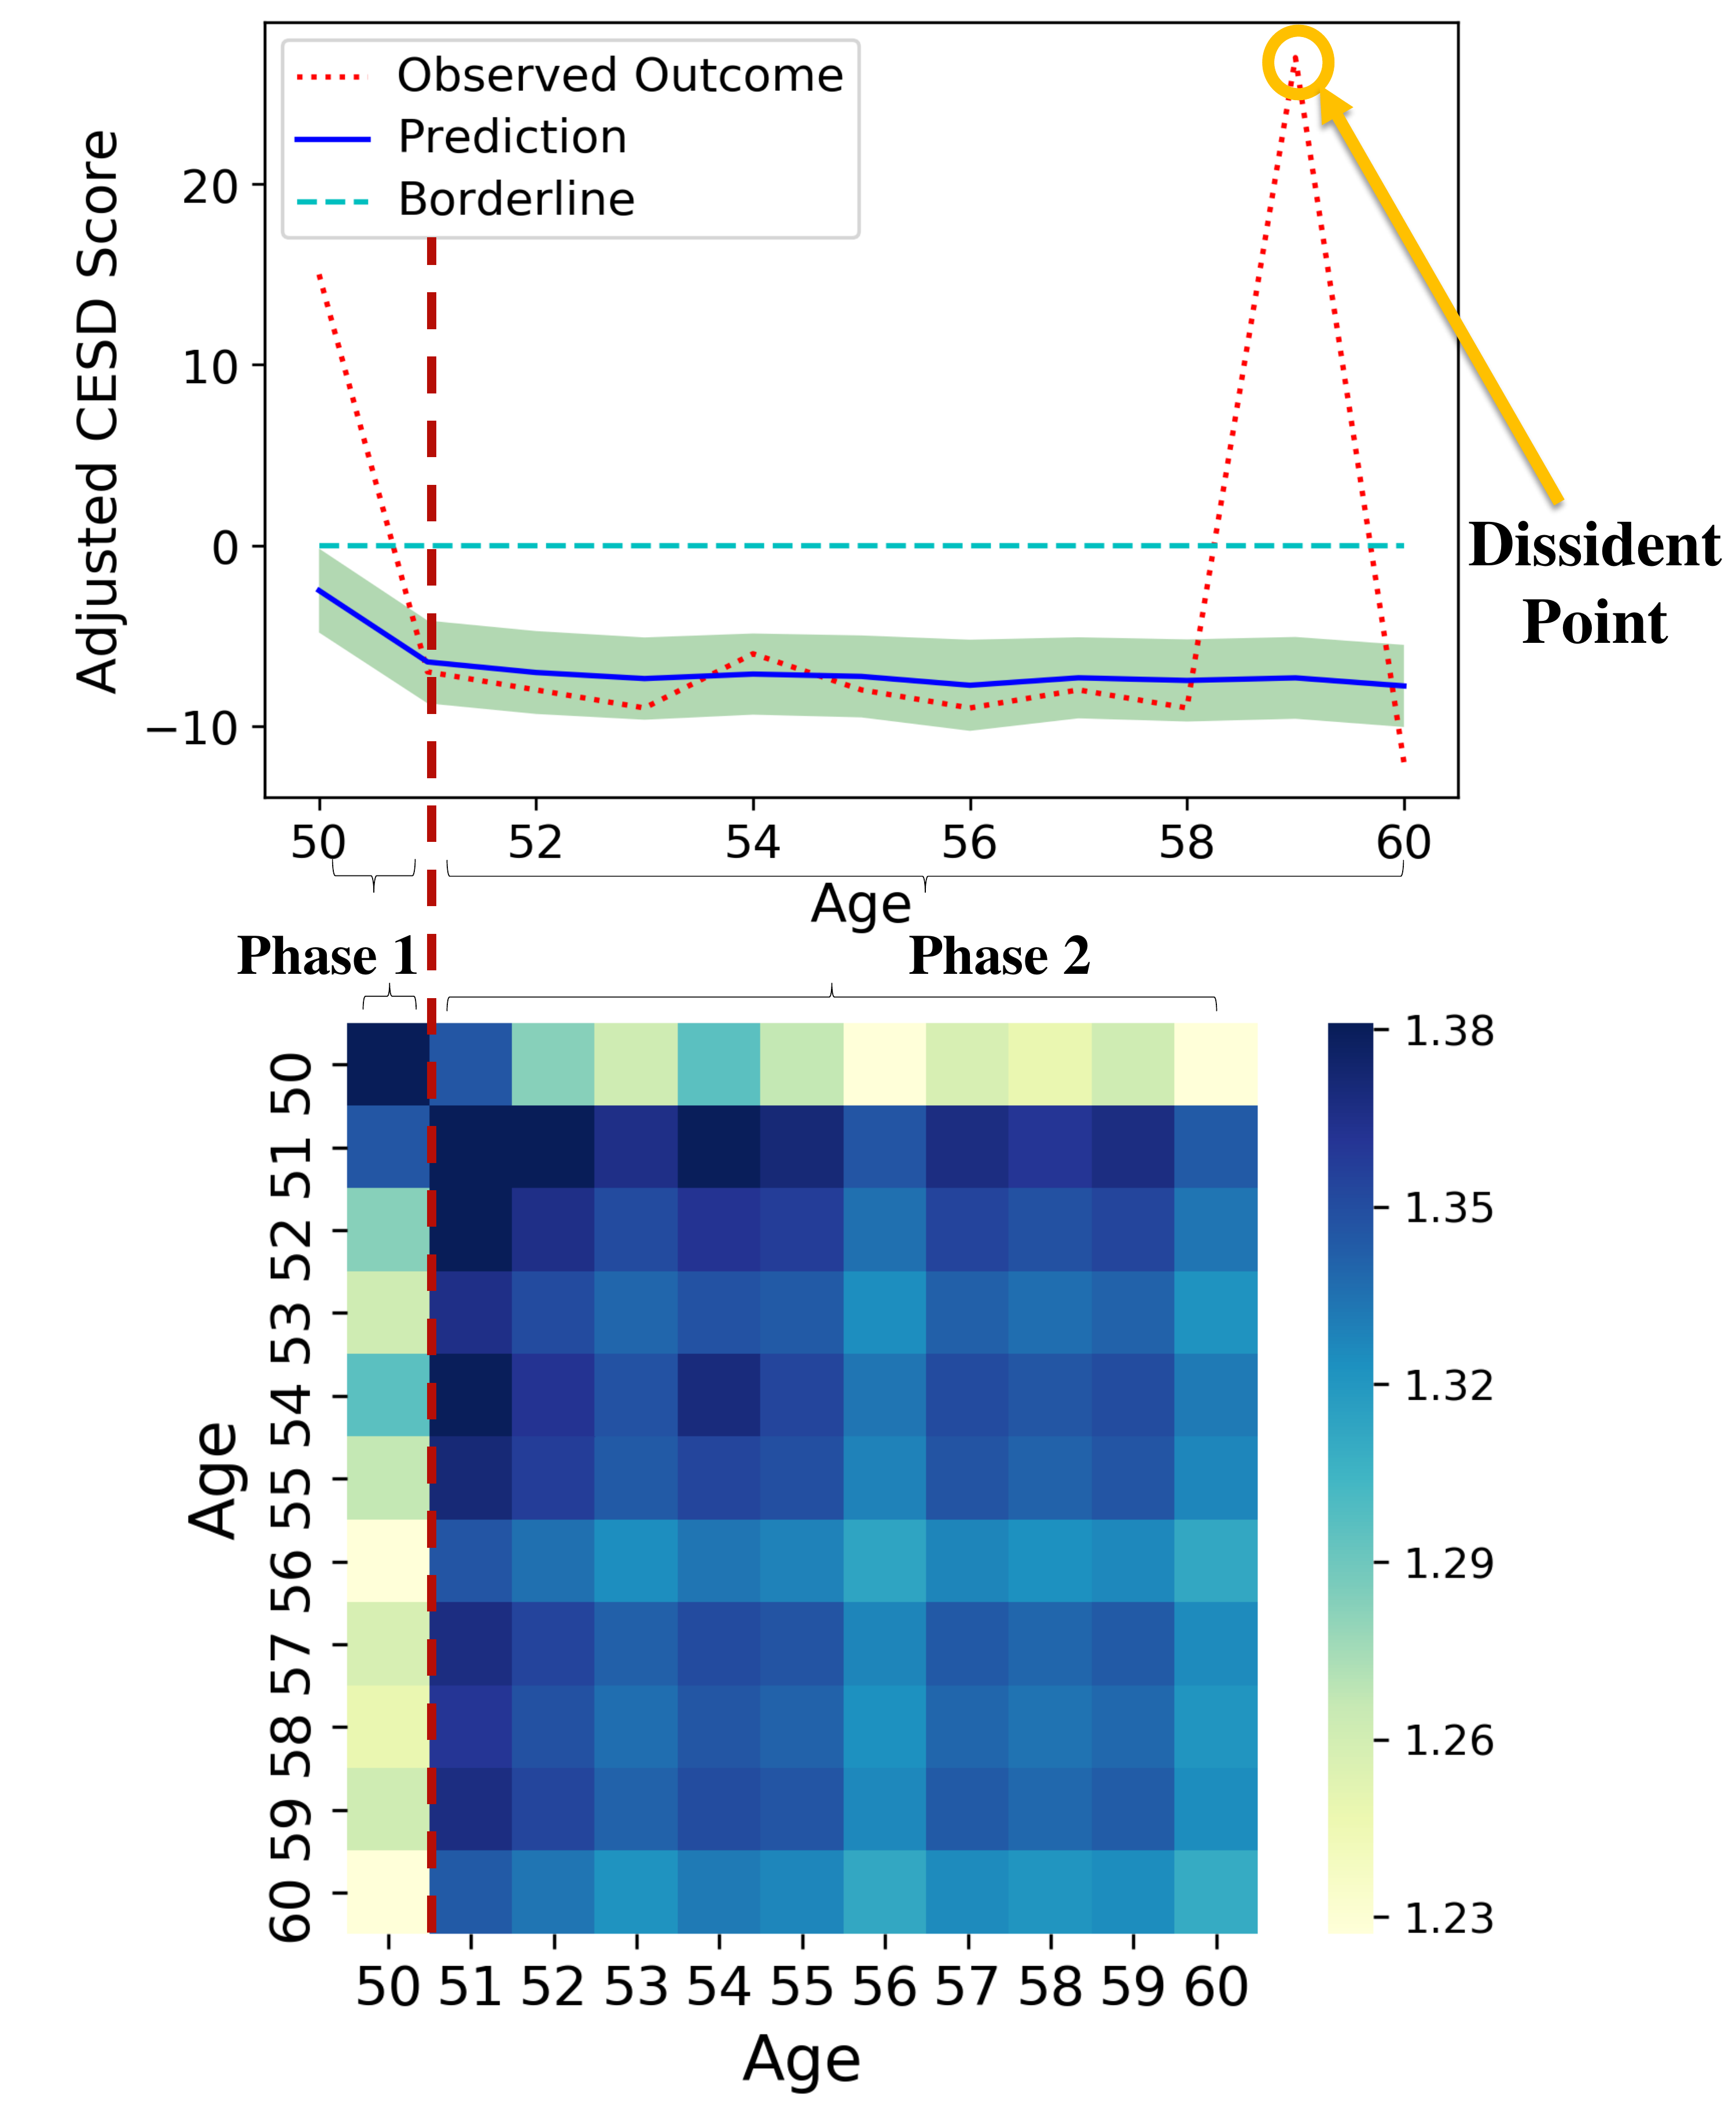}
\label{appfig:individual2}
}
\caption{Case study of two selected individuals from cluster \#1. (Top figures) Observed and predicted trajectories for the adjusted CESD scores; (Bottom figures) Longitudinal correlation among the predictions.}
\label{appfig:swan_case}
\end{figure*}

In the case of real-world data, due to space constraints, we analyze only the correlation structure recovered by L-DKGPR from the SWAN data. Figure~\ref{appfig:swan_cluster_corr} displays the time-invariant cluster correlation after fitting the model to all of the SWAN data. We find that the individuals roughly fall into two clusters, one of which shows a clear cluster structure. The distributions of the adjusted CESD score of the two clusters are shown in Figure~\ref{appfig:swan_cluster_density}. We find that individuals with lower risk of depression tend to be assigned to cluster \#1 whereas those with higher risk of depression tend to be assigned to cluster \#2. Upon examination of the individuals assigned to the two clusters, we can identify at least two individuals that merit further in-depth investigation (See Figure~\ref{appfig:swan_case}). \textbf{Individual \#1}: Judging from the longitudinal correlation as shown in Figure~\ref{appfig:individual1}, we detect a clear transition from absence of depression to depression starting around the age of $52$. Comparison of the covariates between age $52$ and $53$ suggests potential explanations for this transition, e.g., having family and financial issues at $53$ that were not there before age 52. While we have two observations at the age of $55$, the first observation appears to be uncorrelated with the rest, and hence likely to be an outlier. Although the model detects a potential transition from lack of depression to depression, the predictions are consistently below the threshold, suggesting that the individual is by and large not depressive. This could further imply that the depression symptom associated with individual \#1 is likely mild and perhaps temporary. If that is the case,  mental health services could help individual \#1 to successfully overcome what appears to be a temporary depressed phase, likely triggered by family and financial issues. \textbf{Individual \#2}: In the case of  individual \#2 shown in Figure~\ref{appfig:individual2} we  find a  transition from absence of depression to depression around age $50$. The transition is perhaps explained by fact that individual \#2 is experiencing the onset of menopause between the ages of $50$ and $51$. We note that a sudden rise in CESD score  is seen at the age of $59$, which, surprisingly, is consistently ignored by our model. To understand why,  we compare the covariates between age of $58,59$ and $60$. We find no clear evidence  to support the sudden onset of depression. Therefore, we conjecture that the observed adjusted CESD score at $59$ is likely unreliable and a more careful examination might have been warranted.
